# Supplementary material for: MAVIPER: Learning Decision Tree Policies for Interpretable Multi-Agent Reinforcement Learning
Source: arXiv:2205.12449 source file (2022-07-11)
Supplement: Supplementary file 1 [file Appendix.pdf]

**Algorithm 3** VIPER for Single-Agent Setting**Input:**  $(S, A, P, R), \pi^*, Q^*, K, M$ **Output:**  $\hat{\pi}$ 

- 
- 1: Initialize dataset  $\mathcal{D} \leftarrow \emptyset$
  - 2: Initialize policy  $\hat{\pi}^0 \leftarrow \pi^*$
  - 3: **for**  $m = 1$  to  $M$  **do**
  - 4:   Sample  $K$  trajectories:  
 $\mathcal{D}^m \leftarrow \{(s, \pi^*(s)) \sim d^{\hat{\pi}^{m-1}}\}$
  - 5:   Aggregate dataset  $\mathcal{D} \leftarrow \mathcal{D} \cup \mathcal{D}^m$
  - 6:   Resample dataset according to loss:  
 $\mathcal{D}' \leftarrow \{(s, a) \sim p((s, a)) \propto \tilde{l}(s) \mathbb{I}[(s, a) \in \mathcal{D}]\}$
  - 7:   Train decision tree  $\hat{\pi}^m \leftarrow \text{TrainDecisionTree}(\mathcal{D}')$
  - 8: **return** Best policy  $\hat{\pi} \in \{\hat{\pi}^1, \dots, \hat{\pi}^M\}$  on cross validation
- 

**A Omitted Algorithm**

Algorithm 3 shows the full pseudocode for the single-agent version of VIPER [2].

**B Experimental Details****B.1 Environments**

For all environments, we utilize the initialization and reward scheme as described in the original MADDPG paper [20] and Pytorch implementation. The only change we make is to the predator-prey environment, which we describe below.

*Predator-prey.* We follow the definition of the original environment proposed in the multi-agent particle environment [20], with only changes in the partial observation provided to each agent. The observations of the adversary and the agents consist of the concatenation of the following vectors:

1.  $[\text{self\_pos}, \text{self\_vel}]$
2. binarized relative positions and relative velocity (if applicable) of the landmarks and other agents using  $\text{sgn}(x)$  as the binarizing function
3. binarized relative distance between all pairs of agents on the other team. If the opponent team has agent  $a_1, a_2$ , then it will be  $[\text{sgn}(x_1 - x_2), \text{sgn}(y_1 - y_2)]$ .
4. binarized relative distance between all pairs of agents on the same team.

For an environment with  $K = M = 2$ , the observation size will be 22 and 24 respectively for the adversary and the agents.

**B.2 Implementation Details**

To optimize running speed, MAVIPER adopts a caching mechanism to avoid training a new decision tree for each data point being predicted. It also does

parallelization for the `Predict` function starting from Line 23 by precomputing all the prediction information upfront, where the each prediction is delayed until all data points are looped over. In this way, MAVIPER can gather all the predictions that a particular tree needs to make and therefore do it in a parallel manner.

Since IVIPER is fully decentralized, training of each DT can be performed in parallel.

For Fitted Q-Iteration, we bin the states into 10 (mostly) evenly-spaced bins:

$$\begin{aligned} &(-\infty, -1.), [-1., -.75), [-.75, -.5), [-.5, -.25), [-.25, 0.), \\ &[0., .25), [.25, .5), [.5, .75), [.75, 1.), (1., \infty). \end{aligned}$$

We note that Fitted Q-Iteration may perform better with a better choice of bins; however, choosing the correct bin values requires either domain knowledge or extensive manual tuning to find the right balance between granularity, number of timesteps for training, and performance.

### B.3 Hyperparameters

We vary the hyperparameters that would impact training performance of these algorithms 2-3 times and choose the hyperparameters that yield the agents with the best performance. For all environments, we vary the number of rollouts to be  $[50, 100]$  and the number of iterations to be  $[30, 100]$ , while the threshold is fixed at  $N - 1$ . For the baselines, we also vary the maximum number of samples used for training each agent between  $[10000, 30000, 100000]$ . For Imitation DT, we did not see much of a performance increase between 3000 and 10000 samples, so we pick the maximum value for fairness of comparison. For Fitted Q-Iteration, we also did not see much performance increase after 30000 samples, so we chose 30000 samples due to time constraints. Table 2 shows the values of the hyperparameters that are utilized by all algorithms. Although we set a maximum number of training iterations for MAVIPER, we stop training early when there is no noticeable performance gain to further improve runtime.

## C Additional Results

In Appendices C.1 and C.2, we further present results using the defined environment reward. This reward is not as intuitive as the primary metric for many of these environments, but we present the results here for the sake of completeness. The individual and joint performance ratios are defined in the same way as in Section 4.2 in the main body of the paper, with one caveat. Since we are now measuring reward, which may be negative or positive, we take  $\frac{||A| - |B||}{A}$  to report how much more or less  $B$  is than  $A$ .

### C.1 Individual Performance

Figure 6 shows the individual performance ratio measured by reward on all three environments.

| Algorithm          | Environment   | Max Training Iterations | Number of Rollouts | Threshold | Max Samples |
|--------------------|---------------|-------------------------|--------------------|-----------|-------------|
| IVIPER             | Physical      | 50                      | 50                 |           |             |
|                    | Deception     |                         |                    |           |             |
|                    | Cooperative   | 100                     | 50                 | N/A       | 300,000     |
|                    | Navigation    |                         |                    |           |             |
|                    | Predator-prey | 100                     | 100                |           |             |
| MAVIPER            | All           | 100                     | 50                 | $N - 1$   | 300,000     |
| Imitation DT       | All           | 20                      | N/A                | N/A       | 100,000     |
| Fitted Q-Iteration | All           | 10                      | N/A                | N/A       | 30,000      |

Table 2: Hyperparameter values used for all algorithms.

*Physical Deception* Results for physical deception are shown in Figure 6a. Interestingly, MAVIPER and IVIPER defenders only significantly outperform both baselines when the maximum depth is 2. When the maximum depth is 4, MAVIPER, IVIPER, and Imitation DT perform similarly, with Fitted Q-Iteration barely reaching above .50 for all depths. When the maximum depth is 6, Imitation DT actually achieves the highest defender reward, significantly outperforming all other algorithms. However, as shown in Figure 2 in the main body, MAVIPER significantly outperforms all algorithms for all maximum depths when reporting the success ratio. This is because the reward is in part dependent on the performance of the adversary. In other words, a poorly-performing defender can achieve similar performance to a high-performing defender if the poor-performing defender is paired with a high-performing adversary. We see a similar pattern for the adversary performance: IVIPER, MAVIPER, and Fitted Q-Iteration all significantly outperform the Fitted Q-Iteration baseline for different maximum depths. We note that MAVIPER tends to perform better for lower maximum depths, which is desirable for interpretability.

*Cooperative Navigation* Results for cooperative navigation are shown in Figure 6b. IVIPER and MAVIPER significantly outperform the Fitted Q-Iteration baseline for all maximum depths. However, MAVIPER only significantly outperforms Imitation DT when the maximum depth is 2. Otherwise, IVIPER, MAVIPER, and Imitation DT all perform similarly.

*Predator-prey* Results for predator-prey are shown in Figure 6c. MAVIPER prey significantly outperform all other algorithms for maximum depths of 2 and 6. For a maximum depth of 4, MAVIPER and IVIPER algorithms both significantly outperform the baselines. In contrast, MAVIPER predators only significantly outperform all other algorithms for a maximum depth of 4. For a maximum depth of 2, MAVIPER and IVIPER significantly outperform the baselines. For a maximum of depth of 6, MAVIPER, IVIPER, and Imitation DT significantly outperform Fitted Q-Iteration. Again, we note that this performance is not necessarily reflected in the results using the collision metric in Figure 2c.

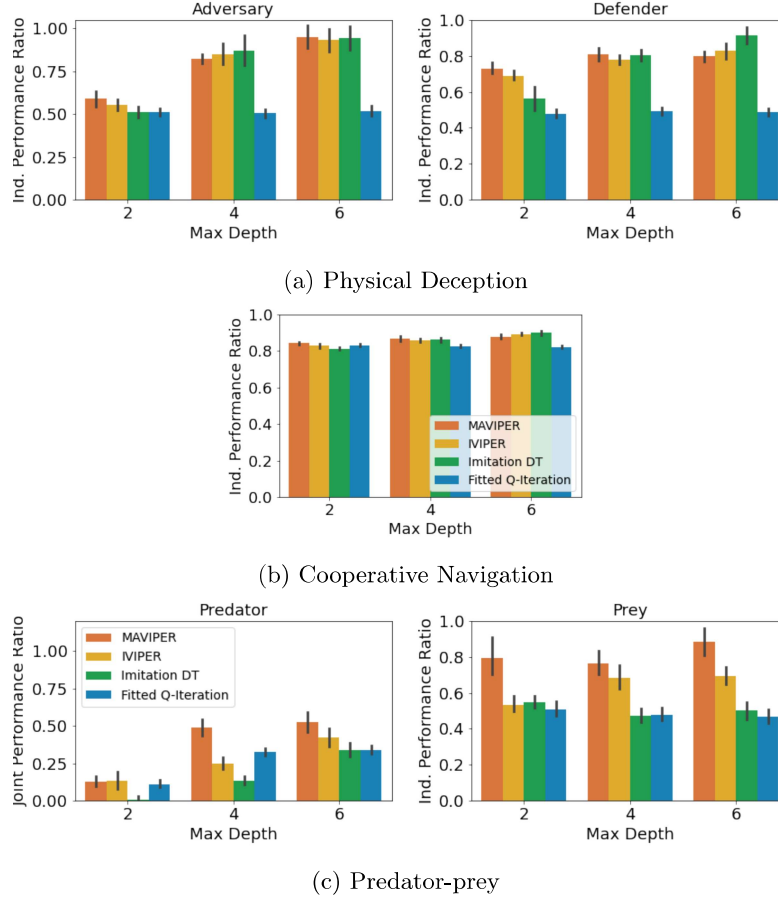

Fig. 6: Individual performance ratio measured by reward. Individual performance ratio of DT agents compared to expert agents for different maximum depths. Higher is better. Error bars represent the 95% confidence interval.

## C.2 Joint Performance

Figure 7 shows the joint performance ratio measured by reward on all three environments.

*Physical Deception* Figure 7a shows the results on physical deception. MAVIPER defenders significantly outperform all other algorithms on this environment for maximum depths of 2 and 4. For a maximum depth of 6, IVIPER, MAVIPER, and Imitation DT all perform similarly. Note that MAVIPER again achieves good performance for lower maximum depths, demonstrating its promise as an algorithm for producing interpretable policies. We also note that, again, the reward metric is somewhat deceptive: when measuring the success conditions in the envi-

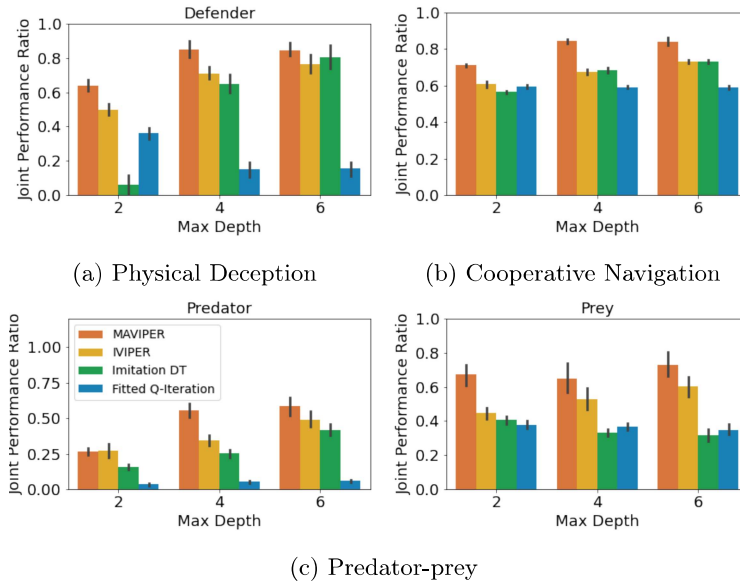

Fig. 7: Joint performance ratio, measured by reward, of DT agents compared to expert agents for different maximum depths. DT agents are evaluated jointly. Error bars represent the 95% confidence interval. Higher is better.

ronment (as in Figure 3 in the main body of the paper), MAVIPER significantly outperforms all other algorithms for all maximum depths.

*Cooperative Navigation* Figure 7b depicts the joint agent performance on the cooperative navigation environment. Interestingly, we see that MAVIPER significantly outperforms all other algorithms for all maximum depths, despite obtaining similar individual performance. Consequently, this means that MAVIPER better captures the desired coordinated behavior than all of the other algorithms.

*Predator-prey* Figure 7c shows the results for the predator-prey environment. MAVIPER prey significantly outperform other algorithms for a maximum depth of 2. For maximum depths of 6 and 8, it achieves slightly better (but not statistically significant) performance than IVIPER, and significantly outperforms the two baselines. MAVIPER and IVIPER predators enjoy similar performance for maximum depths of 2 and 6. For a maximum depth of 4, MAVIPER significantly outperforms all other algorithms. Note that the correct behavior in this environment is challenging to capture with a small decision tree, as the number of features is either 22 or 24, depending on the agent type.

### C.3 Robustness to Different Opponents

We present the full robustness results for the predator-prey and physical deception environments. For space reasons, we only report the average over the

| Predator           | Prey                          |                       |                       |                       |                       |
|--------------------|-------------------------------|-----------------------|-----------------------|-----------------------|-----------------------|
|                    | MAVIPER                       | IVIPER                | Imitation             | Fitted                | MADDPG                |
|                    |                               |                       | DT                    | Q-Iteration           |                       |
| MAVIPER            | ( <b>2.28</b> , <b>2.28</b> ) | ( <b>3.49</b> , 3.49) | ( <b>2.41</b> , 2.41) | ( <b>3.01</b> , 3.01) | ( <b>1.37</b> , 1.37) |
| IVIPER             | (1.95, <b>1.95</b> )          | (2.46, 2.46)          | (2.17, 2.17)          | (2.44, 2.44)          | (0.88, 0.88)          |
| Imitation DT       | (1.32, 1.32)                  | (1.17, <b>1.17</b> )  | (1.18, 1.18)          | (1.40, 1.40)          | (0.61, 0.61)          |
| Fitted Q-Iteration | (0.46, 0.46)                  | (0.30, 0.30)          | (0.24, 0.24)          | (0.18, <b>0.18</b> )  | (0.14, 0.14)          |
| MADDPG             | (2.78, <b>2.78</b> )          | (3.36, 3.36)          | (5.82, 5.82)          | (4.98, 4.98)          | (2.54, 2.54)          |

Table 3: Robustness results of DT agents on predator-prey. Results are presented as: average number of touches in an episode. Higher is better for predator, and lower is better for prey. Excluding MADDPG, the best-performing prey (lowest in value) for each predator type is in **blue** and the best-performing predator (highest in value) for each prey type is in **red**.

| Adversary          | Defender                    |                     |                     |                     |                     |
|--------------------|-----------------------------|---------------------|---------------------|---------------------|---------------------|
|                    | MAVIPER                     | IVIPER              | Imitation           | Fitted              | MADDPG              |
|                    |                             |                     | DT                  | Q-Iteration         |                     |
| MAVIPER            | ( <b>.42</b> , <b>.76</b> ) | ( <b>.45</b> , .33) | (.45, .23)          | ( <b>.37</b> , .01) | (.40, .93)          |
| IVIPER             | (.39, <b>.78</b> )          | ( <b>.45</b> , .32) | (.40, .23)          | ( <b>.38</b> , .00) | (.43, .92)          |
| Imitation DT       | (.40, <b>.79</b> )          | (.42, .34)          | ( <b>.46</b> , .26) | ( <b>.38</b> , .01) | ( <b>.46</b> , .92) |
| Fitted Q-Iteration | (.07, <b>.77</b> )          | (.06, .33)          | (.07, .19)          | (.08, .00)          | (.08, .79)          |
| MADDPG             | (.71, <b>.76</b> )          | (.77, .32)          | (.77, .26)          | (.58, .00)          | (.62, .90)          |

Table 4: Robustness results of DT agents on physical deception. Results are presented as: (adversary success ratio, defender success ratio). Higher is better. Excluding MADDPG, the best-performing defender for each adversary type is in **blue** and the best-performing adversary for each defender type is in **red**.

100 trials; however, we only label the best-performing agent of each type in either **red** or **blue** if the 95% confidence intervals do not overlap, unless otherwise mentioned. We exclude MADDPG from this calculation, since we know that MADDPG agents will outperform all other agent types, and we are mostly interested in how well the *decision tree* policies perform.

*Predator-prey* MAVIPER predators are strictly more robust than all other agents (except MADDPG) to different types of prey. MAVIPER prey are the most or second most robust to different types of predators. In this environment, predator coordination is more critical, as predators must strategically catch the prey. The prey, on the other hand, does not require much coordination, which explains the Imitation DT prey’s robustness by imitating the action of the single-agent expert.

*Physical Deception* MAVIPER defenders are the most robust than all agents (except MADDPG) to different types of adversaries. Interestingly, MAVIPER,

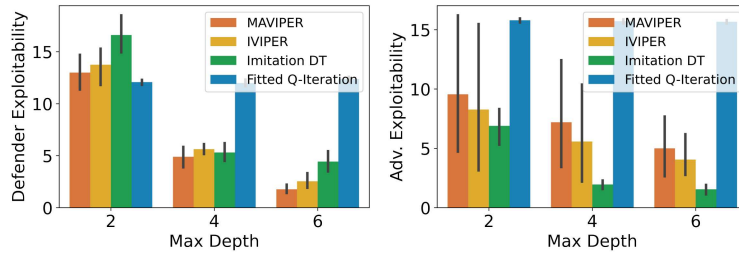

Fig. 8: Exploitability of DT defenders and adversaries in the physical deception environment. Lower exploitability is better.

IVIPER, and Imitation DT adversaries all perform similarly. Indeed, they often do not achieve performance that is statistically significant from one another, as measured by the 95% confidence interval. However, we still highlight the best-performing adversary in red to more easily show the attained performance. Note that MADDPG adversaries can occasionally achieve success greater than around .50, which means that these adversaries can take advantage of some information about the defenders to correctly choose the target to visit. In contrast, adversaries trained with any of the DT-learning algorithms never achieve greater than .50, which indicates that they may need a more complex representation to capture important details about the defenders.

#### C.4 Exploitability

In this set of experiments, we evaluate the exploitability of DT policies in the physical deception environment. Formally, we define the exploitability of a team  $Z$  as:

$$\text{Exploitability of team } Z = \max_{\pi'_{-Z}} U_{-Z}(\pi_Z, \pi'_{-Z}) - U_{-Z}(\pi_Z, \pi_{-Z}), \quad (5)$$

where the optimal  $\pi'_{-Z}$  is the best response policy profile to team  $Z$ 's policies. Practically, to measure exploitability, we fix the policies of the agents in team  $Z$  under evaluation and calculate its approximate best response  $\pi'_{-Z}$  by training a new neural network policy to convergence using MADDPG.

We evaluate the exploitability of the adversary and defenders in the physical deception environment and report the results in Figure 8. For the defending team, MAVIPER exhibits the lowest exploitability on all three depths, showing its effectiveness in learning coordinated policies. It is worth noting that in such a multi-agent learning setting, Imitation DT no longer performs well due to the complexity of the expert and the necessity of cooperation between agents. For the adversary, Imitation DT performs well while IVIPER and MAVIPER performs similarly as the second best. This could be the result that imitation learning quickly imitates a near-optimal expert adversary starting from the depth of four. Since the adversary consists of only a single agent, MAVIPER and IVIPER are reduced to the same method.
